# Supplementary material for: Label Encoding for Regression Networks
Source: arXiv:2212.01927 source file (2022-12-04)
Supplement: Supplementary file 1 [file age.tex]

\newpage
\section{Age Estimation}
\label{sec:a5}
This task aims to predict the age of a person from an image. 
%In this task, the age of a person is predicted from an image. 
We use MORPH-II~\citep{morphii} an AFAD~\citep{agecnn} datasets with data augmentation and evaluation protocols used in ~\citep{mvloss}. 
% trained using the same hyperparameters listed above but without pre-training on Imagenet for even comparison with~\citep{}. 
%We evaluate our predictions using the MAE of the estimated age. 
%e and the CS ($\theta = 5$)\deval{@Fisher: what is CS? what is this $\theta$, we should clarify}. 
%%We use $64$ and $32$ quantization levels for MORPH-II and AFAD datasets and ResNet50 (ImageNet pretrained) as our feature extractor. 
\subsection{Experimental setup}
%Overall, our approach BEL-J results in n $24.9\%$ and $1.73\%$ lower error than direct regression and ORBC. 
We use the MORPH-2~\citep{morphii} and AFAD~\citep{agecnn} datasets for our evaluation. Cumulative Score (CS) and MAE are used as evaluation metrics. We preprocess the MORPH-2 dataset by aligning images first along the average eye position~\citep{mlxtend}, then by re-aligning so that the tip of the nose is in the center of each image. We do not preprocess the AFAD dataset as faces are already centered. Afterwards, face images are resized into $256 \times 256 \times 3$ and randomly cropped to $224 \times 224 \times 3$ for training. For testing, a center crop of $224 \times 224 \times 3$ is taken. 

\paragraph{MORPH-2}
This dataset consists of 55,608 face images with age labels between 16 and 70. The dataset is randomly divided into 39,617 training, 4,398 validation, and 11,001 testing images. 
\paragraph{AFAD}
This dataset consists of 164,432 Asian facial images and age labels between 15 and 40. The dataset is randomly divided into 118,492 training, 13,166 validation, and 32763 testing images. 
\paragraph{Training parameters}
We performed two runs with different random seeds to determine the learning rate between $[0.00001, 0.0001, 0.001]$ and use a batch size of 64 for all experiments. We use ImageNet pretrained weights to initialize the network. 
\begin{table}[h]
    \begin{center}
      \setlength\tabcolsep{6pt}
      \caption{Training parameters for age estimation using MORPH-II and AFAD dataset }
      \label{tab:trage}
      \footnotesize
      \begin{tabular}{L{3cm}C{1cm}ccC{2cm}C{2cm}}
        \toprule
       Optimizer & Epochs & Batch size &  Learning rate & Learning rate schedule  \\  \midrule
      Adam, weight decay=0, momentum=0 & 50 & 64 & 0.0001 & 1/10 at 30, 40 epochs
      \\ \bottomrule
      \end{tabular}
    \end{center}
    \end{table}
\subsection{Related work}
Existing approaches for age estimation include ordinal regression~\citep{agecnn, coralcnn}, soft regression~\citep{ssrnet}, and expected value ordinal regression ~\citep{mvloss, dldl}. OR-CNN~\citep{agecnn} proposed the use of ordinal regression via binary classification to predict the label. CORAL-CNN~\citep{coralcnn} refined this approach by enforcing the ordinality of the model output. SSR-Net~\citep{ssrnet} proposed the use of stage-wise soft regression using the softmax of the classification output to refine the predicted label. MV-Loss~\citep{mvloss} extended the soft regression approach by penalizing the output of the model based on the variance of the age distribution, while DLDL~\citep{dldl} proposed to use the KL-divergence between the softmax output and a generated label distribution to train a model. 
\subsection{Evaluation}
%%%%
\begin{table}[]
  \centering
  \footnotesize
  \caption{Comparison of BEL design parameters on MAE for age estimation for MORPH-II dataset and ResNet50 feature extractor.}
  \label{tab:edlmorph}
  \begin{tabular}{C{2cm}C{1.5cm}rrrrrr}
  \toprule
& \multicolumn{1}{c}{} & \multicolumn{6}{c}{Encoding function}     \\ \cline{3-8} 
  Decoding function   & Loss function                & \multicolumn{1}{l}{U} & \multicolumn{1}{l}{J} & \multicolumn{1}{l}{B1JDJ} & \multicolumn{1}{l}{B2JDJ} & \multicolumn{1}{l}{HEXJ} & \multicolumn{1}{l}{HAD} \\ \midrule
  BEL-J/BEL-U & BCE & 2.32 & \textbf{2.27} & - & - & - & - \\\hline
  GEN-EX & BCE & 2.30 & 2.29 & 2.35 & 2.49 & 2.45 & 2.99 \\\hline
  GEN & BCE & 2.28 & 2.28 & 2.34 & 2.51 & 2.54 & 3.07 \\\hline
  GEN-EX & CE & 2.55 & 2.54 & 2.75 & 2.65 & 2.63 & 12.33 \\\hline
  GEN & CE & 2.60 & 2.58 & 2.61 & 2.66 & 2.61 & 3.10 \\\hline
  GEN-EX & L1 & 2.30 & 2.30 & 2.32 & 2.30 & 2.32 & 2.29 \\
  \bottomrule        
  \end{tabular}
  \end{table}
  %%%%
Table~\ref{tab:edlmorph} compares different combinations of encoding, deocding, and loss functions for BEL approach on MORPH-II dataset and ResNet50 feature extractor. 
\begin{table}[h]
    {
    \centering
    \setlength\tabcolsep{4pt}
    \caption{Age estimation results on MORPH-II dataset. $\theta=10$ is used for BEL.}
    \label{tab:age}
    \footnotesize
    \begin{tabular}{L{4.4cm}cR{2cm}L{2cm}L{2cm}}
    \toprule
    Approach & Feature extractor & \#Parameters (M) & MORPH-II (MAE)& MORPH-II (CS$\theta = 5$)\\ \midrule
    OR-CNN~\citep{agecnn} (Ordinal regression by binary classification ) & - & 1.0 & 2.58 & 0.71 \\ \hline
    MV Loss~\citep{mvloss} (Direct regression) & VGG-16 & 138.4 & 2.41 & 0.889 \\ \hline
    DLDL-v2~\citep{dldl} (Ordinal regression with multi-class classification) & ThinAgeNet & 3.7 & \underline{1.96}* & - \\ \hline
    CORAL-CNN~\citep{coralcnn} (Ordinal regression by binary classification) & ResNet34 & 21.3 & 2.49 & - \\ \hline \hline
    Direct Regression (L2 Loss) & ResNet50 & 23.1 & 2.44 $\pm$ 0.01 & 0.903 $\pm$ 0.002 \\ \hline
    BEL-J/BCE/BEL-J & ResNet50 & 23.1 & \textbf{{2.27}} $\pm$ 0.01& \textbf{\underline{0.928}} $\pm$ 0.001\\   \bottomrule 
    \end{tabular}
    }
    \scriptsize{\\\*Uses custom data augmentation for the training}
    %\vspace{-3mm}
\end{table}
\begin{table}[]
  \centering
  \footnotesize
  \caption{Comparison of BEL design parameters on MAE for age estimation for AFAD dataset and ResNet50 feature extractor.}
  \label{tab:edlafad}
  \begin{tabular}{C{2cm}C{1.5cm}rrrrrr}
  \toprule
& \multicolumn{1}{c}{} & \multicolumn{6}{c}{Encoding function}     \\ \cline{3-8} 
  Decoding function   & Loss function                & \multicolumn{1}{l}{U} & \multicolumn{1}{l}{J} & \multicolumn{1}{l}{B1JDJ} & \multicolumn{1}{l}{B2JDJ} & \multicolumn{1}{l}{HEXJ} & \multicolumn{1}{l}{HAD} \\ \midrule
  BEL-J/BEL-U & BCE & 3.13 & 3.15 & - & - & - & - \\\hline
GEN-EX & BCE & 3.14 & 3.16 & 3.32 & 3.35 & 3.28 & 3.34 \\\hline
GEN & BCE & 3.13 & 3.19 & 3.41 & 3.44 & 3.41 & 3.52 \\\hline
GEN-EX & CE & 3.26 & 3.29 & 3.38 & 3.44 & 3.40 & 3.30 \\\hline
GEN & CE & 3.36 & 3.34 & 3.42 & 3.47 & 3.40 & 3.45 \\\hline
GEN-EX & L1 & 3.13 & 3.12 & \textbf{3.11} & 3.12 & 3.13 & 3.13 \\
  \bottomrule        
  \end{tabular}
  \end{table}
  %%%%
Table~\ref{tab:edlafad} compares different combinations of encoding, deocding, and loss functions for BEL approach on AFAD dataset and ResNet50 feature extractor. 
\begin{table}[h]
  {
  \centering
  \setlength\tabcolsep{4pt}
  \caption{Age estimation results on AFAD dataset. $\theta=10$ is used for BEL.}
  \label{tab:agee}
  \footnotesize
  \begin{tabular}{L{4.4cm}cR{2cm}L{2cm}L{2cm}}
  \toprule
  Approach & Feature extractor & \#Parameters (M) & AFAD (MAE)& AFAD (CS$\theta = 5$)\\ \midrule
  OR-CNN~\citep{agecnn} (Ordinal regression by binary classification ) & - & 1.0 & 3.51 & 0.74 \\ \hline
  CORAL-CNN~\citep{coralcnn} (Ordinal regression by binary classification) & ResNet34 & 21.3 & 3.47 & - \\ \hline \hline
  Direct Regression (L2 Loss) & ResNet50 & 23.1 & 3.21 $\pm$ 0.02 & 0.810 $\pm$ 0.02 \\ \hline
 BEL-B1JDJ/MAE/GEN-EX & ResNet50 & 23.1 & \textbf{\underline{3.11}} $\pm$ 0.01& \textbf{\underline{0.823}} $\pm$ 0.001\\ \bottomrule 
  \end{tabular}
  }
  %\vspace{-3mm}
\end{table}
Table~\ref{tab:age} and Table~\ref{tab:agee} compare \BEL{ }with other regression approaches for MORPH-II and AFAD datasets. 
%BEL-J achieves $17.7\%$ nd $4.3\%$ improvement over direct regression and domain-specific regression approaches, respectively. 
BEL-x provides lower MAE than the direct regression for both datasets, and BEL-B1JDJ/MAE/GEN-EX results in the lowest MAE for the AFAD dataset compared to the state-of-the-art approaches. 
OR-CNN~\citep{agecnn} and CORAL-CNN~\citep{coralcnn} use ordinal regression by binary classification approach. We achieve significant improvement over these approaches due to the differences in encoding and decoding function, regressor architecture, and training framework. This improvement shows the potential of these  design aspects to improve regression accuracy.
