# Supplementary material for: Label Encoding for Regression Networks
Source: arXiv:2212.01927 source file (2022-12-04)
Supplement: Supplementary file 2 [file auto.tex]

\newpage
\section{End-to-end Autonomous Driving}
\label{sec:a6}
We evaluate our approach on the NVIDIA PilotNet dataset for end-to-end autonomous driving~\citep{pilotold}. 
In this task, the steering wheel's next angle is predicted from an image of the road. 

\subsection{Experimental setup}
End-to-end autonomous driving is the problem of predicting the target wheel state directly from an image representing the view in front of a car. We use a driving dataset consisting of 45,500 images taken around Rancho Palos Verdes and San Pedro, California~\citep{sully}. We crop images to $256\times 70\times 3$ then resized them to $200\times 66\times 3$. We randomly vary the brightness of the image between $[0.2\times, 1.5\times]$ and randomly perturb the steering direction.
We use PilotNet architecture~\citep{pilotnet} and use $\theta=10$ with $670$ quantization levels for \BEL.  
\paragraph{Training parameters}
We performed two runs with different random seeds to determine the learning rate between $[0.00001, 0.0001, 0.001, 0.01, 0.1]$ and use a batch size of 64 for all experiments. 
\begin{table}[h]
    \begin{center}
      \setlength\tabcolsep{6pt}
      \caption{Training parameters for end-to-end autonomous driving using PilotNet. }
      \label{tab:trage}
      \footnotesize
      \begin{tabular}{L{3cm}C{2cm}ccC{2cm}C{2cm}}
        \toprule
       Optimizer & Epochs & Batch size &  Learning rate & Learning rate schedule  \\  \midrule
       SGD with weight decay=1e-5, momentum=0 & 50 & 64 & 0.1 & 1/10 at 10, 30 epochs
      \\ \bottomrule
      \end{tabular}
    \end{center}
    \end{table}
\subsection{Related work}
End-to-end autonomous driving is a novel task that has become increasingly relevant due to the rise of self-driving vehicles. The autonomous driving model's task is to predict the future driving angle based on a forward-facing image from the perspective of the vehicle. PilotNet~\citep{pilotnet} used a small, application-specific network to succeed within the latency constraints of autonomous driving.
%Explaining How a Deep Neural Network Trained with End-to-End Learning Steers a Car
\subsection{Evaluation}
\begin{table}[]
  \centering
  \footnotesize
  \caption{Comparison of BEL design parameters on MAE for end-to-end autonomous driving for PilotNet dataset and feature extractor.}
  \label{tab:edlpilot}
  \begin{tabular}{C{2cm}C{1.5cm}rrrrrr}
  \toprule
& \multicolumn{1}{c}{} & \multicolumn{6}{c}{Encoding function}     \\ \cline{3-8} 
  Decoding function   & Loss function                & \multicolumn{1}{l}{U} & \multicolumn{1}{l}{J} & \multicolumn{1}{l}{B1JDJ} & \multicolumn{1}{l}{B2JDJ} & \multicolumn{1}{l}{HEXJ} & \multicolumn{1}{l}{HAD} \\ \midrule
  BEL-J/BEL-U & BCE & 4.34 & 3.91 & - & - & - & - \\ \hline
  GEN-EX & BCE & 4.57 & 4.20 & 4.83 & 4.96 & 5.29 & 10.12 \\ \hline
  GEN & BCE & 4.37 & 3.95 & 3.51 & 3.61 & 4.01 & 10.00 \\ \hline
  GEN-EX & CE & 4.30 & 4.16 & 4.99 & 5.87 & 5.39 & 87.17 \\ \hline
  GEN & CE & 3.15 & \textbf{3.11} & 3.14 & 3.21 & 3.64 & 6.20 \\ \hline
  GEN-EX & L1 & 4.10 & 4.11 & 4.34 & 4.34 & 4.11 & 5.09 \\
  \bottomrule        
  \end{tabular}
  \end{table}
  %%%%
Table~\ref{tab:edlpilot} compares different combinations of encoding, deocding, and loss functions for BEL approach on PilotNet dataset and  feature extractor. 
Table~\ref{tab:pilot} compares binary encoded labels with the PilotNet which uses direct regression~\citep{pilotnet}.
\BEL-x results in a significant reduction in the MAE compared to the direct regression approach. 
\begin{table}[h]
    {
    \begin{center}
    \setlength\tabcolsep{4pt}
    \caption{End-to-end autonomous driving results on PilotNet dataset and architecture~\citep{pilotnet,pilotold}.}
    \label{tab:pilot}
    \footnotesize
    \begin{tabular}{L{5.3cm}ccc}
    \toprule
    Approach & Feature extractor & \#Parameters (M) & MAE \\ \midrule
    PilotNet~\citep{pilotnet} & PilotNet & 1.8 & 4.24 $\pm$ 0.45 \\ \hline
    BEL-J/GEN/CE & PilotNet & 1.8 & \textbf{\underline{3.11}} $\pm$ 0.01 \\ 
    \bottomrule 
    \end{tabular}
    \end{center}
    }
\end{table}
