# Supplementary material for: Label Encoding for Regression Networks
Source: arXiv:2212.01927 source file (2022-12-04)
Supplement: Supplementary file 4 [file hpe.tex]

\newpage
\section{Head Pose Estimation}
\label{sec:a3}
Head pose estimation aims to find a human head's pose in terms of three angles: yaw, pitch, and roll. 
In this work, we consider landmark-free 2D head pose estimation. 
We use two evaluation protocols, Protocol-1 (Train dataset: 300W-LP~\citep{300wlp}, Test dataset: AFLW2000~\citep{aflw}) and Protocol-2 (70-30\% train-test split of BIWI dataset~\citep{biwi}) with mean absolute error (MAE) as the evaluation metric. 

Head pose estimation aims to find a human head's pose in terms of three angles: yaw, pitch, and roll. 
This work considers landmark-free 2D head pose estimation, which performs the task based on RGB image information without using facial landmark information. 
\subsection{Experimental setup}
We use two evaluation protocols with three widely used datasets: 300W-LP~\citep{300wlp}, BIWI~\citep{biwi}, AFLW2000~\citep{300wlp} and follow the evaluation setting of Hopenet~\citep{hopenet} and FSA-Net~\citep{fsanet}.
Mean absolute error (MAE) is used as the evaluation metric and the individual yaw, pitch, and roll and overall MAE are evaluated. NVIDIA 2080Ti GPU is used for all the experiments. 
Bold numbers represent the lowest error for the same feature extractor and data augmentation, and the
underlined numbers represent the lowest error overall. Evaluation metrics for BEL and direct regression are
averaged over five training runs with random seeds.
We further explain two protocols in detail. 

Bold numbers represent the lowest error for the same feature extractor and data augmentation, and the
underlined numbers represent the lowest error overall. Evaluation metrics for BEL and direct regression are
averaged over five training runs with random seeds.
\paragraph{Protocol 1:} In this setting, the synthetic 300W-LP dataset is used for training, consisting of $122,450$ samples. The trained network is tested on a real-world AFLW2000 dataset. Yaw, pitch, and roll angles are in the range $[-99,99]$ for both datasets. Table~\ref{tab:trp1} provides a summary of the training parameters. 
\begin{table}[h]
    \begin{center}
      \setlength\tabcolsep{3pt}
      \caption{Training parameters for head pose estimation with protocol 1. }
      \label{tab:trp1}
      \footnotesize
      \begin{tabular}{L{3cm}C{2cm}cC{1cm}C{1.5cm}C{2cm}C{1.5cm}}
        \toprule
      Approach & Optimizer & Epochs & Batch size &  Learning rate & Learning rate schedule  & Training time (GPU hours) \\  \midrule
      ResNet50 with direct regression and BEL & Adam, weight decay=0, momentum = 0 & 20 & 16 & 0.00001 & 1/10 after 10 Epochs & 4 \\ \hline
      RAFA-Net with direct regression~\citep{rafanet} and BEL & RMSProp, momentum=0, rho = 0.9 & 100 & 16 & 0.001 & - & 48 \\ 
      \bottomrule
      \end{tabular}
    \end{center}
    \end{table}
For head pose estimation with ResNet50 architecture (Direct regression and \BEL), two runs with different random seeds for each combination of learning rate $\{0.001,0.0001,0.00001\}$ and batch size $\{8,16\}$ are used for hyperparameter tuning. For data augmentation, images are loosely cropped around the center in the training and testing datasets with random flipping and blurring. Samples with angles in the range [$-99^{\circ}$,$99^{\circ}$] are considered for training and testing. $200$ quantization levels for binary-encoded labels.

For head pose estimation with RAFA-Net, we use the training parameters used in~\citep{rafanet}. 
For data augmentation, we use the approach used in the previous work on RAFA-Net for head pose estimation using direct regression. Angles in the range [$-180^{\circ}$,$180^{\circ}$] with 360 quantization levels are considered for BEL. 

\paragraph{Protocol 2:} BIWI dataset is used for training and evaluation in this protocol. BIWI dataset consists of $24$ videos of $20$ subjects with total $15,128$ frames. Three random splits of 70\%-30\% images are used for training and evaluation. Table~\ref{tab:trp2} provides a summary of the training parameters. 

For head pose estimation with ResNet50 architecture (Direct regression and \BEL), two runs with different random seeds for each combination of learning rate $\{0.001,0.0001,0.00001\}$ and batch size $\{8,16\}$ are used for hyperparameter tuning. For data augmentation, images are loosely cropped around the center in the training and testing datasets with random flipping. 
For the BIWI dataset, the yaw angle is in the range $[-75,75]$, the pitch is in the range $[-65,85]$, and the roll angle is in the range $[-55,45]$. Total $150$ quantization levels are used for yaw and pitch, and $100$ quantization levels are used for roll. 

For head pose estimation with RAFA-Net, we use the training parameters used in~\citep{rafanet}. 
For data augmentation, we use the approach used in the previous work on RAFA-Net for head pose estimation using direct regression. Angles in range [$-180^{\circ}$,$180^{\circ}$] with 360 quantization levels are considered for BEL. 
\begin{table}[h]
  \begin{center}
    \setlength\tabcolsep{3pt}
    \caption{Training parameters for head pose estimation with protocol 1. }
    \label{tab:trp2}
    \footnotesize
    \begin{tabular}{L{3cm}C{2cm}cC{1cm}C{1.5cm}C{2cm}C{1.5cm}}
      \toprule
    Approach & Optimizer & Epochs & Batch size &  Learning rate & Learning rate schedule  & Training time (GPU hours) \\  \midrule
    ResNet50 with direct regression and BEL & Adam, weight decay=0, momentum = 0 & 50 & 8 & 0.0001 & 1/10 after 30 Epochs & 2 \\ \hline
    RAFA-Net with direct regression~\citep{rafanet} and BEL & RMSProp, momentum=0, rho = 0.9 & 100 & 16 & 0.001 & - & 6 \\ 
    \bottomrule
    \end{tabular}
  \end{center}
  \end{table}
\subsection{Related work}
Existing approaches for head pose estimation includes stage-wise soft regression~\citep{ssrnet,fsanet}, combination of classification and regression~\citep{deepheadpose,hopenet}, and ordinal regression~\citep{quatnet}. 
%Head pose estimation has seen significant success from ordinal regression methods, where the model must predict the pose of a human head given an image. This pose is generally represented with 3 degrees of freedom (pitch, yaw, roll). 
SSR-Net~\citep{ssrnet} proposed the use of stage-wise soft regression that uses softmax values of classification output to refine the label. 
FSA-Net ~\citep{fsanet} proposes extending stage-wise estimation to head pose estimation using feature aggregation. 
HopeNet~\citep{hopenet} uses a combination of classification and regression loss to train a model for head pose estimation. 
Whereas QuatNet~\citep{quatnet} solves head pose estimation using a combination of regression L2 loss and ordinal regression loss. 
RAFA-Net~\citep{rafanet} uses an attention based approach for feature extraction with direct regression. 
%Hyperface~\citep{hyperface}, TCDCN~\citep{tcdcn} demonstrates that head pose estimation can be learned jointly with other tasks to improve performance.
\subsection{Evaluation}
\paragraph{Protocol 1 (HPE2 and HPE4)}
%%% EDL for COFW
\begin{table}[]
  \centering
  \footnotesize
  \caption{Comparison of BEL design parameters on MAE for head pose estimation with ResNet50 feature extractor.}
  \label{tab:edl1resnet}
  \begin{tabular}{C{2cm}C{1.5cm}rrrrrr}
  \toprule
& \multicolumn{1}{c}{} & \multicolumn{6}{c}{Encoding function}     \\ \cline{3-8} 
  Decoding function   & Loss function                & \multicolumn{1}{l}{U} & \multicolumn{1}{l}{J} & \multicolumn{1}{l}{B1JDJ} & \multicolumn{1}{l}{B2JDJ} & \multicolumn{1}{l}{HEXJ} & \multicolumn{1}{l}{HAD} \\ \midrule
  BEL-J/BEL-U & BCE & 4.78 & 4.84 & - & - & - & - \\ \hline
  GEN-EX & BCE & \textbf{4.77} & 4.84 & 5.43 & 5.09 & 4.94 & 7.84 \\\hline
  GEN & BCE & 4.78 & 4.87 & 5.11 & 5.05 & 5.15 & 8.54 \\\hline
  GEN-EX & CE & 4.93 & 5.04 & 5.04 & 4.97 & 4.79 & 5.64 \\\hline
  GEN & CE & 5.07 & 5.17 & 5.13 & 5.10 & 4.99 & 5.62 \\\hline
  GEN-EX & L1 & 5.05 & 5.18 & 5.19 & 5.09 & 5.17 & 5.07 \\ \bottomrule        
  \end{tabular}
  \end{table}
  %%%%
  \begin{table}[]
    \centering
    \footnotesize
    \caption{Comparison of BEL design parameters on MAE for head pose estimation with RAFA-Net feature extractor.}
    \label{tab:edl1rafanet}
    \begin{tabular}{C{2cm}C{1.5cm}rrrrrr}
    \toprule
  & \multicolumn{1}{c}{} & \multicolumn{6}{c}{Encoding function}     \\ \cline{3-8} 
    Decoding function   & Loss function                & \multicolumn{1}{l}{U} & \multicolumn{1}{l}{J} & \multicolumn{1}{l}{B1JDJ} & \multicolumn{1}{l}{B2JDJ} & \multicolumn{1}{l}{HEXJ} & \multicolumn{1}{l}{HAD} \\ \midrule
    BEL-J/BEL-U & BCE & 3.94 & 4.00 & - & - & - & - \\\hline
    GEN-EX & BCE & \textbf{3.90} & 3.93 & 10.42 & 15.40 & 29.11 & 9.17 \\\hline
    GEN & BCE & 3.93 & 3.94 & 4.21 & 4.25 & 4.53 & 9.21 \\\hline
    GEN-EX & CE & 4.55 & 4.62 & 4.34 & 4.53 & 4.45 & 5.12 \\\hline
    GEN & CE & 4.68 & 4.75 & 4.46 & 4.61 & 4.63 & 5.29 \\\hline
    GEN-EX & L1 & 4.45 & 5.87 & 5.11 & 9.34 & 10.43 & 17.89 \\\hline
    \bottomrule        
    \end{tabular}
    \end{table}
    %%%%
Table~\ref{tab:edl1resnet} compares different combinations of encoding, deocding, and loss functions for BEL approach on protocol 1 and ResNet50 feature extractor. 
Table~\ref{tab:edl1rafanet} compares different combinations of encoding, deocding, and loss functions for BEL approach on protocol 1 and RAFA-Net feature extractor. 
Table~\ref{tab:hpe1} shows results for protocol 1 with error margin for 95\% confidence interval. For ResNet50 feature extractor, BEL-U/BCE/GEN-EX provides the lowest MAE compared to direct regression and HopeNet~\citep{hopenet}. Whereas, for RAFA-Net feature extractor, BEL-U/BCE/GEN-EX provides the lowest MAE compared to direction regression (L2 loss).   
\begin{table}[h]
  \begin{center}
  \setlength\tabcolsep{6pt}
  \caption{Landmark-free 2D Head poses estimation evaluation for protocol 1.  $200$ and $360$ quantization levels are used for \BEL{ }with ResNet50 and RAFA-Net. } 
  \label{tab:hpe1}
  \footnotesize
  \begin{tabular}{L{3.2cm}C{1.4cm}C{1.1cm}llll@{}}
    \toprule
    Approach & Feature Extractor  & \#Params (M) &  Yaw & Pitch & Roll & MAE  \\ \midrule
  SSR-Net-MD~\citep{ssrnet} { }{ }  (Soft regression) & SSR-Net & 1.1 & 5.14 & 7.09 & 5.89 & 6.01 \\ \hline
  FSA-Caps-Fusion~\citep{fsanet} (Soft regression)  & FSA-Net & 5.1 & 4.50 & 6.08 & 4.64 & 5.07  \\  \hline \hline
  HopeNet* ($\alpha$ = 2)~\citep{hopenet} (classification + regression loss) &  ResNet50 &  23.9 & 6.47 & 6.56 & 5.44 & 6.16 \\ \hline
  Direct regression (L2 loss) & ResNet50 & 23.5  &  6.34 & 6.90 & 6.87  & 6.71 $\pm$ 0.13   \\ \hline
  BEL-U/BCE/GEN-EX  & ResNet50 & 23.6 & \textbf{4.54} & \textbf{5.76} & \textbf{3.96}  & \textbf{4.77} $\pm$ 0.05  \\  \hline \hline
  RAFA-Net~\citep{rafanet} (Direct Regression)  & RAFA-Net & 69.8 & 3.60 & {{4.92}} & 3.88 & 4.13 \\ \hline 
  BEL-U/BCE/GEN-EX  & RAFA-Net & 69.8 &\textbf{\underline{3.28}} & \textbf{\underline{4.78}} & \textbf{\underline{3.55}} & \textbf{\underline{3.90}} $\pm$ 0.03 \\
 \bottomrule
  %\cmidrule(r){1-4}
  \end{tabular}\\
  \scriptsize{$*$uses different data preprocessing}
\end{center}
  \end{table}
\paragraph{Protocol 2 (HPE1 and HPE3)}
%%% EDL for COFW
\begin{table}[]
  \centering
  \footnotesize
  \caption{Comparison of BEL design parameters on MAE for head pose estimation with ResNet50 feature extractor.}
  \label{tab:edl2resnet}
  \begin{tabular}{C{2cm}C{1.5cm}rrrrrr}
  \toprule
& \multicolumn{1}{c}{} & \multicolumn{6}{c}{Encoding function}     \\ \cline{3-8} 
  Decoding function   & Loss function                & \multicolumn{1}{l}{U} & \multicolumn{1}{l}{J} & \multicolumn{1}{l}{B1JDJ} & \multicolumn{1}{l}{B2JDJ} & \multicolumn{1}{l}{HEXJ} & \multicolumn{1}{l}{HAD} \\ \midrule
  BEL-J/BEL-U & BCE & 3.38 & 3.65 & - & - & - & - \\\hline
  GEN-EX & BCE & \textbf{3.37} & 3.64 & 5.11 & 8.02 & 4.76 & 7.53 \\\hline
  GEN & BCE & 3.38 & 3.65 & 5.16 & 8.16 & 4.99 & 7.73 \\\hline
  GEN-EX & CE & 4.22 & 3.55 & 3.88 & 4.08 & 4.09 & 5.50 \\\hline
  GEN & CE & 4.25 & 3.62 & 3.93 & 4.06 & 4.39 & 5.48 \\\hline
  GEN-EX & L1 & 3.81 & 3.93 & 3.66 & 3.59 & 5.99 & 4.21 \\ \bottomrule        
  \end{tabular}
  \end{table}
  %%%%
  %%% EDL for COFW
\begin{table}[]
  \centering
  \footnotesize
  \caption{Comparison of BEL design parameters on MAE for head pose estimation with RAFA-Net feature extractor.}
  \label{tab:edl2rafa}
  \begin{tabular}{C{2cm}C{1.5cm}rrrrrr}
  \toprule
& \multicolumn{1}{c}{} & \multicolumn{6}{c}{Encoding function}     \\ \cline{3-8} 
  Decoding function   & Loss function                & \multicolumn{1}{l}{U} & \multicolumn{1}{l}{J} & \multicolumn{1}{l}{B1JDJ} & \multicolumn{1}{l}{B2JDJ} & \multicolumn{1}{l}{HEXJ} & \multicolumn{1}{l}{HAD} \\ \midrule
  BEL-J/BEL-U & BCE & 3.47 & 3.16 & - & - & - & - \\\hline
  GEN-EX & BCE & 3.46 & \textbf{3.12} & 11.67 & 13.29 & 25.42 & 5.75 \\\hline
  GEN & BCE & 3.49 & 3.14 & 3.62 & 3.78 & 4.44 & 5.83 \\\hline
  GEN-EX & CE & 3.82 & 3.91 & 3.52 & 3.49 & 3.98 & 3.98 \\\hline
  GEN & CE & 3.92 & 4.09 & 3.62 & 3.65 & 4.35 & 4.28 \\\hline
  GEN-EX & L1 & 3.72 & 3.60 & 4.31 & 4.29 & 6.61 & 18.69 \\ \bottomrule        
  \end{tabular}
  \end{table}
  %%%%
Table~\ref{tab:edl2resnet} compares different combinations of encoding, deocding, and loss functions for BEL approach on protocol 2 and ResNet50 feature extractor. 
Table~\ref{tab:edl2rafa} compares different combinations of encoding, deocding, and loss functions for BEL approach on protocol 2 and RAFA-Net feature extractor. 
Table~\ref{tab:hpe2} shows results for protocol 2 with error margin for 95\% confidence interval. For ResNet50 feature extractor, BEL-U/BCE/GEN-EX provides the lowest MAE compared to direct regression (L2 loss). Whereas, for RAFA-Net feature extractor, BEL-J/BCE/GEN-EX provides the lowest MAE compared to direction regression (L2 loss). For both the feature extractors, \BEL{ } results in significant decrease in the MAE for pitch compared to direct regression. 
\begin{table}[t]
  \begin{center}
  \setlength\tabcolsep{6pt}
  \caption{Landmark-free 2D Head poses estimation evaluation for protocol 2.  $150$ and $360$ quantization levels are used for \BEL{ }with ResNet50 and RAFA-Net. } 
  \label{tab:hpe2}
  \footnotesize
  \begin{tabular}{L{3.2cm}C{1.4cm}C{1.1cm}llll@{}}
    \toprule
    Approach & Feature Extractor  & \#Params (M) &  Yaw & Pitch & Roll & MAE  \\ \midrule
  SSR-Net-MD~\citep{ssrnet} { }{ }  (Soft regression) & SSR-Net & 1.1  & 4.24  & 4.35 & 4.19 & 4.26 \\ \hline
  FSA-Caps-Fusion~\citep{fsanet} (Soft regression)  & FSA-Net & 5.1 & 2.89 & 4.29 & 3.60 & 3.60    \\  \hline \hline
  Direct regression (L2 loss) & ResNet50 & 23.5  &  4.62  & 5.24  & 4.43 & 4.76 $\pm$ 0.35  \\ \hline
  BEL-U/BCE/GEN-EX  & ResNet50 & 23.6  & \textbf{3.28} & \textbf{\underline{3.36}}  & \textbf{3.44}  & \textbf{3.37} $\pm$ 0.09\\  \hline \hline
  RAFA-Net~\citep{rafanet} (Direct Regression)  & RAFA-Net & 69.8 & 3.07 & 4.30 & 2.82 & 3.40 
 \\ \hline 
  BEL-J/BCE/GEN-EX  & RAFA-Net & 69.8 & \textbf{\underline{2.83}} & \textbf{{3.82}} & \textbf{\underline{2.70}}& \textbf{\underline{3.12}} $\pm$ 0.12\\
  \bottomrule
  %\cmidrule(r){1-4}
  \end{tabular}
\end{center}
\end{table}
\newpage
